# Supplementary material for: Computation of the correlated metal-insulator transition in vanadium dioxide from first principles
Source: arXiv:1310.1066 source file (2015-01-31)
Supplement: Supplementary file 1 [file supplementary.pdf]

# Supplementary Material of “Characterization of the correlated metal-insulator transition in vanadium dioxide from first-principles”

Huihuo Zheng and Lucas K. Wagner

Department of Physics, University of Illinois at Urbana-Champaign Urbana, IL 61801-3080, USA

## I. DFT BAND STRUCTURES WITH HYBRID FUNCTIONALS

Fig.SM 1 shows the DFT band structures of different exchange-correlation functionals.

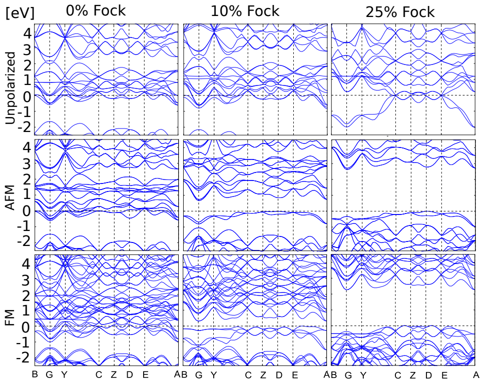


(a)Rutile

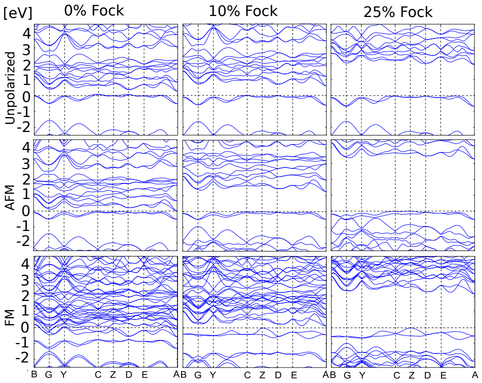


(b)Monoclinic

FIG.SM 1. DFT band structures of different exchange-correlation functionals. For FM states, both of the two spin channels (spin majority and spin minority) are plotted on the figure. Three different mixing of Hartree-Fock are used in the computations, 0%, 10% and 25%.

## II. PSEUDOPTENTIAL, FINITE SIZE, AND TIMESTEP ERRORS

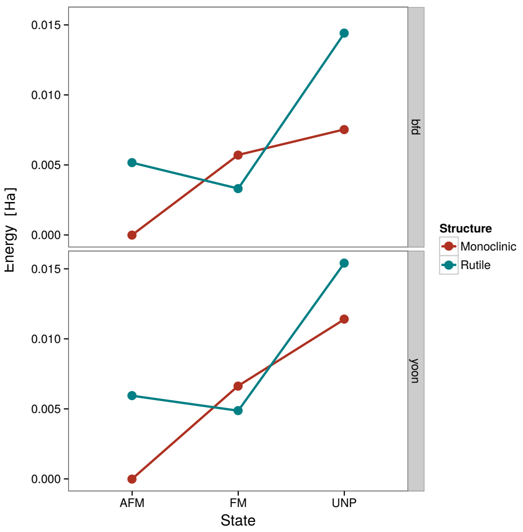


(a)

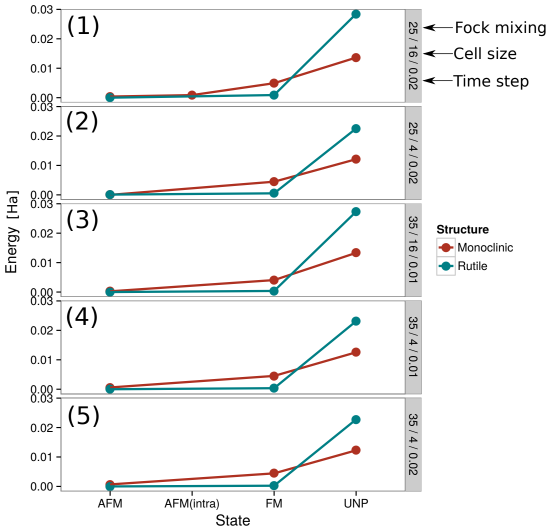


(b)

FIG.SM 2. Pseudoptential, finite size, and timestep error analysis: (a) Energetic results of 4-$VO_2$ cells for different pseudopotentials: BFD and Yoon. PBE functional was employed in DFT to optain the trial wave function for FN-DMC. (b) Energetic results of different cell size, time step and different hybrid functionals. BFD pseudopotential was used in (1)-(5).

We computed fixed-node diffusion quantum Monte Carlo (FN-DMC) energy for two different supercells (4-$VO_2$ cell and 16-$VO_2$ cell), with different timestep (0.02 $Ha^{-1}$ and 0.01 $Ha^{-1}$.), and with different pseudopotentials (BFD and Yoon). Noted from Fig.SM. 2(a), the two different pseudopotentials show qualitatively same behavior. We should mention that in DFT level, both the two pseudopotentials give the same band structure that is in agreement with all electron calculations. Compare Fig.SM. 2(b)(1) and (2), we find that for PBE0 functional, 4-$VO_2$ cell and 16-$VO_2$ cell give us the same results (the difference is within stochastical errorbars). Compare Fig.SM 2(b)(4) and (5), we also find that if a time step of 0.02 $Ha^{-1}$ already give us converged results.

## III. FN-DMC COMPUTATIONS OF OPTICAL GAPS

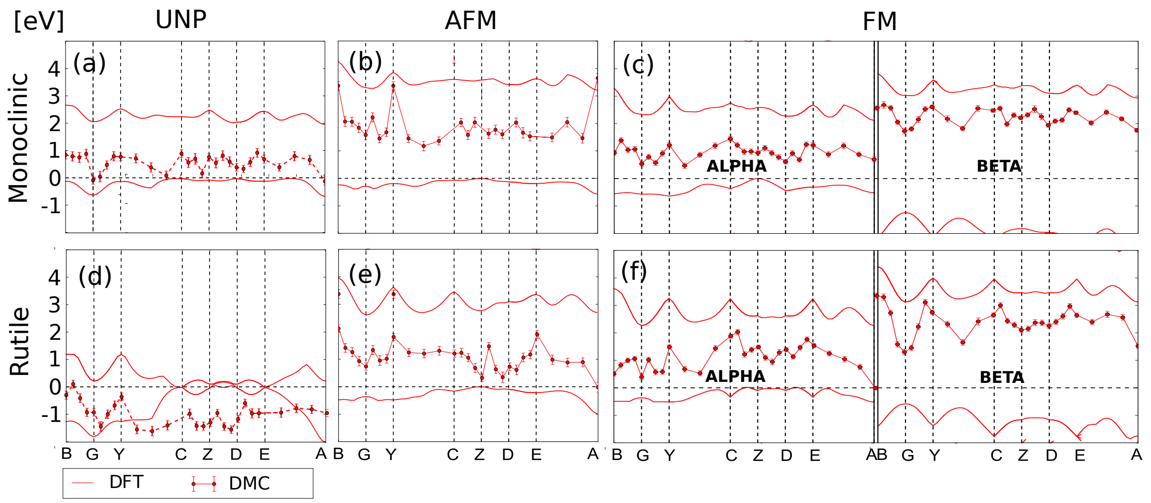


FIG.SM 3. Quasiparticle band structures of $VO_2$ in different phases. These band structures correspond to a unit cell containing 4 $VO_2$ formula units. The DFT functional used is PBE0.

Fig.SM 3 shows the optical excitation by FN-DMC. We compute the FN-DMC energy gap by replacing the highest occupied Kohn-Sham orbital with unoccupied ones and compute the energy change from the original ground state.

## IV. PSEUDOPOTENTIAL AND BASIS SET

In order for other people to reproduce our results, we herein provide the pseudopotential and basis set used in our calculations in CRYSTAL input format.

**Vanadium**

```
223 11
INPUT
13.0 3 1 1 0 0 0
    2.163618   13.000000 −1
    4.079018   28.127028 1
    3.214364  −48.276563 0
    8.443260   96.232266 0
    6.531361   41.580435 0
0 0 6 2.0 1.0
  18.360298 −0.023212
  11.577461 0.200288
  6.390046 −0.55432
  1.528787 0.565283
  0.72883 0.543474
  0.349741 0.134989
0 0 6 0.0 1.0
  18.360298 0.002873
  11.577461 −0.043911
  6.390046 0.144148
  1.528787 −0.165823
  0.72883 −0.313756
  0.349741 −0.055699
0 2 6 6.0 1.0
  13.883264 0.003648
  6.174 −0.175046
  4.772897 0.155473
  2.182411 0.346594
  1.049492 0.44341
  0.49268 0.263803
0 3 4 1.0 1.0
  7.384196 0.067593
  3.350355 0.246802
  1.398721 0.336404
  0.571472 0.349348
0 4 1 0.0 1.0
  0.850084 1.0
0 1 1 0. 1.
  0.2 1. 1.
0 1 1 0. 1.
  0.6 1. 1.
0 1 1 0. 1.
  1.8 1. 1.
0 3 1 0. 1.
  0.2 1.
0 3 1 0. 1.
  0.6 1.
0 3 1 0. 1.
  1.8 1.
```

**Oxygen**

```
208 6
INPUT
6.0 3 1 0 0 0 0
    9.297939    6.000000 −1
    8.864922   55.787634 1
    8.629257  −38.819785 0
    8.719245   38.419141 0
0 0 7 2.0 1.0
  0.573098 0.453752
  1.225429 0.295926
  2.620277 0.019567
  5.602818 −0.128627
  11.980245 0.012024
  25.616801 0.000407
  54.775216 −7.6e−05
0 2 7 6.0 1.0
  0.333673 0.255999
  0.666627 0.281879
  1.331816 0.242835
  2.660761 0.161134
  5.315785 0.082308
  10.620108 0.039899
  21.217318 0.004679
0 3 1 0.0 1.0
  0.66934 1.0
0 1 1 0. 1.
  0.2 1. 1.
0 1 1 0. 1.
  0.6 1. 1.
0 1 1 0. 1.
  1.8 1. 1.
```
